# Supplementary material for: Market Potential for CO$_2$ Removal and Sequestration from Renewable Natural Gas Production in California
Source: arXiv:2105.01644 ancillary file (2021-05-04)
Supplement: Supplementary file 1 [file si.pdf]

# Supplemental Information for "Market Potential for $CO_2$ Removal and Sequestration from Renewable Natural Gas Production in California"

Jun Wong
UC Berkeley, Environmental Science, Policy, and Management

Jonathan Santoso
UC Berkeley, Chemical and Biomolecular Engineering

Marjorie Went
UC Berkeley, Chemical and Biomolecular Engineering

Daniel Sanchez*
UC Berkeley, Environmental Science, Policy, and Management

July 2020

## More on data development

We filter the NATCARB saline aquifer database to only sequestration sites with nonurban layers using urban area definitions from (1) and the (2). We further filter the NATCARB database using a depth to basement of 1500m to ensure the safety of $CO_2$ sequestered. Depth to basement is obtained from the (3). We use a conservative measure of depth to basement (as opposed to 800m) to allow for the uncertainty of the policy directive regarding CCS in California. We filter the data available from Breunig et al. (4) to those flagged as suitable for anaerobic digestion. In particular, we do not consider the more lignin-rich feedstocks that are less prone to anaerobic digestion. While biogas from gasification is a studied and relatively mature technology, we constrain this paper to biogas from anaerobic digestion (5). The hand-collected data on existing anaerobic digesters are then geocoded using the Google Maps Place API (6).

We linearize the cost functions obtained from the literature. Specifically, we estimate the piecewise linear functions of the digester and upgrading cost functions in Parker et al. (7), compression and pumping cost in McCollum and Ogden (8), and carbon dioxide capture cost in Psarras et al. (9). Piecewise estimating non-linear functions allows us to better capture the economies of scale associated with CCS systems and stay within the framework of linear optimization. This reduces the model complexity and computational load while still approximating the importance of scale in CCS systems. We employ the cost model in Psarras et al. (9) to estimate the cost of $CO_2$ capture, assuming a 90% capture rate and 80.7% $CO_2$ concentration.

## Biogas yields

While we use the biogas yields in Li et al. (10) at baseline, we also survey the literature for a broad range of experimental biogas yields for sensitivity analysis. See Table A1 for the range of biogas yields considered and sources surveyed. In addition, we adopt the predictive biogas yield model from Escalante et al.

*Corresponding author: sanchezd@berkeley.edu. Code and replication kit can be found on GitHub.

Table A1: Literature Biogas Yield (mL/g VS)

| Feedstock | Min | Max |
|---|---|---|
| Manure | 51 | 295 |
| Crop Waste | 49 | 390 |
| Food Waste | 180 | 540 |
| Green Waste | 180 | 540 |
| Grease | 648 | 811 |

Table A2: Biogas Yield Prediction Model Coefficient

| Panel A: Model Coefficients | |
|---|---|
| Variable | Coefficient |
| Cellulose | 0.3445 |
| Hemicellulose | 0.0001 |
| Lignin | -0.0001 |
| C:N ratio | -0.0002 |
| Percent Volatile Solids | -0.0040 |
| Percent Total Solids | 0.0012 |
| Inoculum:Substrate ratio | -0.00002 |

| Panel B: Average Estimated Yields (mL/g VS) | |
|---|---|
| Feedstock | Biogas Yield |
| Crop Residues | 181.96 |
| Food Waste | 328.78 |
| Manure | 324.32 |

(11) to supplement the literature values. We consider six independent variables: cellulose, hemicellulose, and lignin weight percentage; C:N ratio; and volatile and total solids percentage and the inoculum to substrate ratio. Table A2 panel A, presents coefficients for each predictive variable and panel B presents the estimated biogas yields for select feedstocks.

Unsurprisingly, Figure A1 shows that $CH_4$ and $CO_2$ output is the most sensitive to biogas yield asumptions. Under optimistic biogas yield assumptions, over 150 PJ of RNG is produced and 6 million tons of CO2 is sequestered at baseline policy support. Using more pessimistic biogas yield assumptions, only 40 PJ of RNG is produced and 1.5 million tons of CO2 sequestered. Despite this, biogas yield has little effect on profits in the model, with policy drivers such as LCFS and RFS driving most of the variation.

This discussion on biogas yield requires two caveats: this model aggregates feedstock types into broad categories. Biogas yield varies within the broad categories presented in the paper, and considering the average biogas yield for all subtypes of biomass residues masks the variation in feedstock subtype availability across regions. In particular, agricultural production is relatively segregated in California: while Fresno primarily produce almonds and tomatoes, neighboring Tulare leads in orange production (12). The different climate in California implies that there will be important regional differences in available crop residues. Breunig et al. (4) provides more detail on the geographic (and temporal) variation in biomass residues across California. Second, special attention needs to be paid to codigesting facilities. In particular, while codigestion have the potential to further increase the biogas yield, it is also possible that biogas yield could be dampened due to an inappropriate mixture of feedstocks. In this paper, we assume that feedstocks are mixed homogenously, and their respective biogas yields aggregate linearly.

Figure A1: Sensitivity Analysis

(a) $CH_4$ Sensitivity

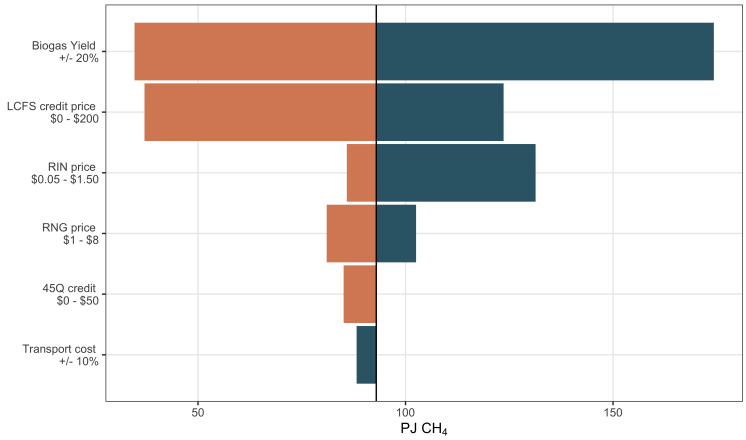


(b) $CO_2$ Sensitivity

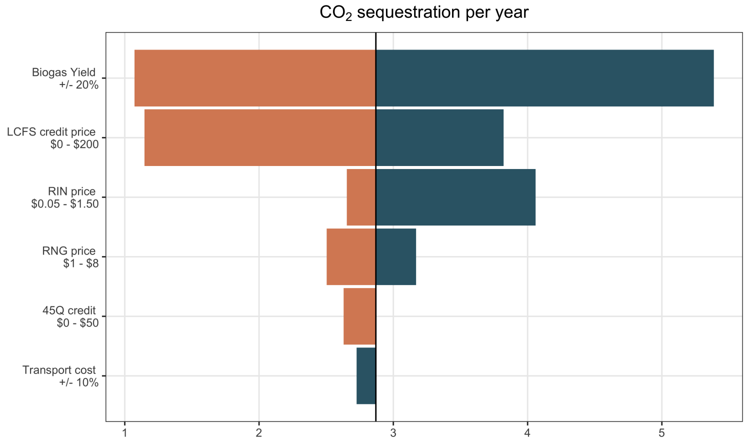

Figure A2: Cost and Revenues

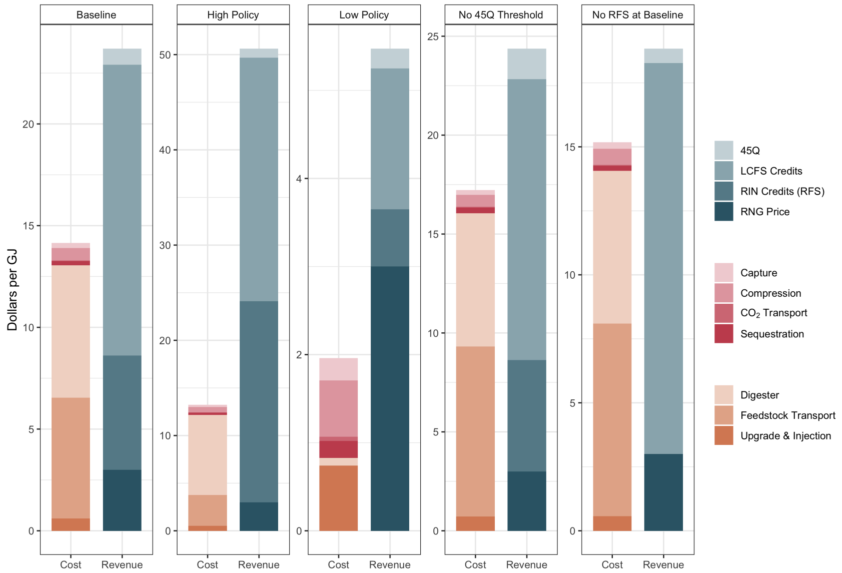


# Biogas upgrading technologies

In this paper, we consider pressure swing adsorption (PSA) for biogas upgrading. There are other technologies available, with varying $CH_4$ and $CO_2$ purity and costs. We briefly discuss the implications of various technologies while we direct interested readers to Sun et al. (13) and Ong et al. (14) for an in-depth overview of biogas upgrading technologies. Among the various biogas upgrading technologies, water scrubbing, pressure swing adsorption, and chemical scrubbing are the most commonly applied technologies (14). In particular, PSA is relatively inexpensive and is widely practiced. It also requires no heat demand and low energy use. It's applicability to small capacities is especially helpful in our context. Water scrubbing is similarly inexpensive, but it requires large amounts of water to operate and requires biomethane drying. Chemical scrubbing, unlike PSA and water scrubbing, yields higher methane content, but it is relatively more expensive and difficult to operate. The costs of upgrading technologies are varied, but PSA is consistently one of the lower cost options across case studies. The choice of biogas upgrading technology could be consequential to the model outcomes. In particular, what is the trade off between the purity of $CH_4$ and $CO_2$ streams, the energetic content of the resulting natural gas, and the cost of technology? However, the results in Figure A2 suggests that the upgrading costs are relatively small compared to digester cost or CCS-related costs.

# Sequestration costs

We determine the sequestration storage costs following Sanchez et al. (15). In particular, saline aquifer storage and capacity and location are derived from NATCARB v1502 (16). Discussed above, we extend the approach in Sanchez et al. (15) by further filtering for depth to basement past 1500m and sequestration sites in non-urban areas. Storage costs are estimated for each 10km by 10km grids. The cost of site characterization is based on areal footprint, well drilling and completion, injection equipment, operating and maintenance costs, and monitoring and verification costs (17, 18). We estimate the capacity-weighted levelized cost of sequestration for each site using the following equation:

$$C_{seq} = (CRF \times \frac{C_{well,D\&C} + C_{well,equip} + C_{well,O\&M} + C_{seismic}}{q_{well,max}} + CRF \times \frac{C_{char}}{q_{annual}} + C_{mon}) \times Q_{normalized} \tag{1}$$

where
$C_{seq}$ = levelized cost of $CO_2$ (\$/ton)
$CRF$ = capital recovery factor $C_{well,D\&C}$ = cost of drilling and completion
$C_{well,equip}$ = cost of well equipment
$C_{well,O\&M}$ = cost of well operation and maintenance
$C_{seismic}$ = cost of seismic assessment and monitoring
$C_{char}$ = site characterization cost
$C_{mon}$ = monitoring and verification cost
$q_{well,max}$ = maximum well injection rate
$q_{annual}$ = annual injection volume
$Q_{normalized}$ = normalized saline aquifer capacity

The maximum well injection rate is asssumed to be 1 $MtCO_2$/y. We update the cost to 2018 US dollars using the IHS Upstream Capital Cost Index. We estimate the cost of seismic assessment and monitoring from C2SAFE. In particular, seismic assessment costs \$160,000/$km^2$ of site area, and a constant 10 percent of total seismic cost for processing field data. Note that the characterization costs depend on the size of the aerial footprint, estimating as the following (19):

$$C_{char} = C_{areal,char} \times \lambda_c \times q_{annual} \times \frac{t}{\Psi \times b \times \lambda_w} \tag{2}$$

where
$C_{areal,char}$ = specific site characterization costs
$q_{annual}$ = annual injection volume (at reservoir conditions)
$\lambda_c$ = phase mobility of $CO_2$[1]
$\lambda_w$ = phase mobility of brine
$t$ = period of injection
$b$ = $CO_2$ layer thickness
$\Psi$ = porosity

We estimate the physical properties needed for $CO_2$ and brine phase mobilities using Chung et al. (20) and Batzle and Wang (21), respectively. We include a \$52 million per site to account for development costs based on McCollum and Ogden (8). We assume a cost of monitoring and verification of \$0.1/$tCO_2$.

# Additional results

Figure A3 shows that at baseline, a majority of available feedstocks are utilized, except for food waste. The current policy incentive is sufficient to spark a profitable, carbon negative, waste management program in California. However, the relatively small utilization of food waste points to the importance of transportation costs. However, the outsized profitability of the RNG-CCS system indicates that it is possible to further manage food waste in a similar manner while maintaining a profitable system.

Figure A4 shows the geographical distribution of facility level cost at baseline. We see the landfills are consistently less expensive than codigesters, this is because landfills lack the need for an anaerobic digester. There is a lower-cost agglomeration in the greater Los Angeles area, while Imperial county sees a higher-cost cluster. Furthermore, cost is directly correlated with facility size—the smallest facilities are the most expensive (on a dollars-per-GJ basis). Note that such an uneven distribution of levelized cost across regions and facilities is only possible through a global optimization. Whereas a local optimization problem might see a significant decline in system size.

[1]The phase mobility is the ratio of relative permeability to fluid viscosity

Figure A3: Feedstock utilization

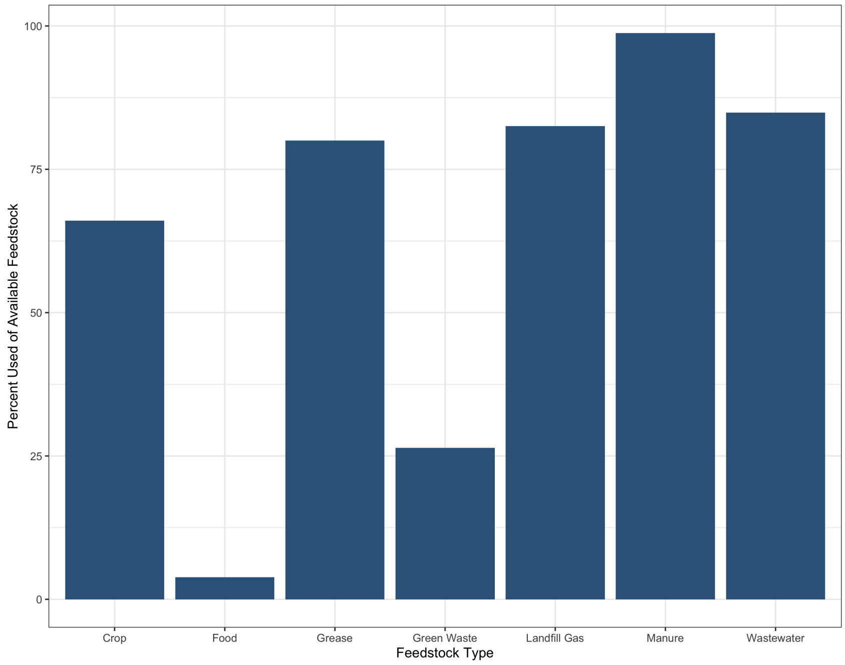


Figure A4: Levelized Cost

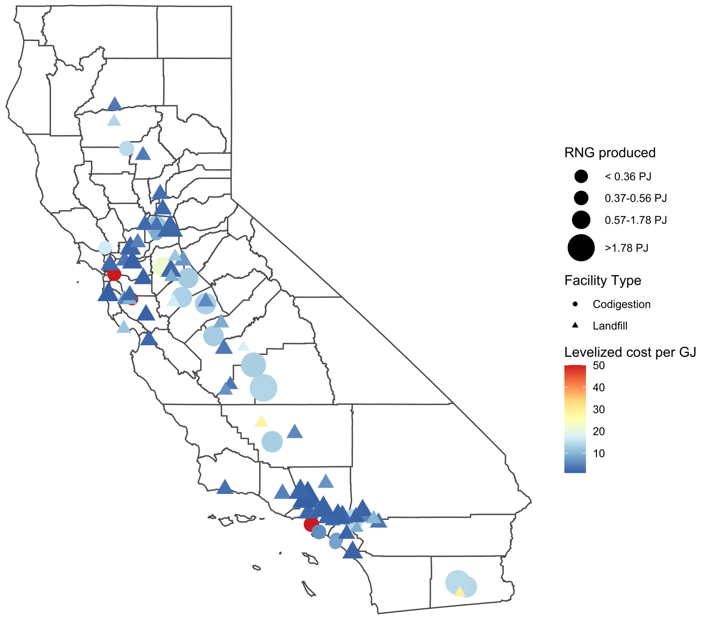

# Model Formulation

## Notation

Sets are as follows:

| | |
|---|---|
| $f$ | Facilities |
| $l \in f$ | Landfills, a subset of facilities |
| $c \in f$ | Codigesters, a subset of facilities |
| $t$ | Feedstock type |
| $g \in t$ | Landfill gas, a subset of feedstock type |
| $s \in t$ | Set of codigestion types, subset of feedstock type |
| | $s = \{$Wastewater, Crop, Manure, MSW$\}$ |
| $i$ | Sequestration sites |
| $s$ | Feedstock source |
| $(s, f)$ | Feedstock source and facility pairs under 50 miles |
| $(f, i)$ | Facility and sequestration site pairs under 50 miles |

Parameters are as follows:

| | |
|---|---|
| **Facilities** | |
| $\text{pipe\_fc}_f$ | RNG pipeline fixed cost at facility $f$ |
| $\text{pipe\_vc}_f$ | RNG pipeline variable cost at facility $f$ |
| $\text{lmop}_l$ | Landfill collecting variable cost at landfill $l$ |
| | |
| **Sequestration sites** | |
| $\text{injection\_fc}_i$ | $CO_2$ injection fixed cost at sequestration site $i$ |
| $\text{injection\_vc}_i$ | $CO_2$ injection variable cost at sequestration site $i$ |
| $\text{capacity}_i$ | Sequestration site storage capacity at sequestration site $i$ |
| $\text{seismic}_i$ | 3-D seismic survey cost at sequestration site $i$ |
| | |
| **Type** | |
| $\text{ts}_t$ | Total solids % of feedstock type $t$ |
| $\text{vs}_t$ | Volatile solids % of feedstock type $t$ |
| $\text{ton}_t$ | Conversion to ton of feedstock type $t$ |
| $\text{biogas\_yield}_t$ | Biogas yield of feedstock type $t$ |
| $\text{c\_intensity}_t$ | Carbon intensity of resultant RNG from feedstock type $t$ |
| | |
| **Feedstock source & type** | |
| $\text{supply}_{s,t}$ | Feedstock quantity at source $s$ of type $t$ |
| | |
| **Valid source → facility pairs** | |
| $\text{fs\_dist}_{s,f}$ | Road distance between feedstock at location $s$ and facility $f$ |
| $\text{fs\_time}_{s,f}$ | Travel duration between feedstock at location $s$ and facility $f$ |
| $\text{per\_ton}_{s,f}$ | Per-ton cost from location $s$ to facility $f$ |
| | |
| **Valid facility → sequestration site pairs** | |
| $\text{rs\_dist}_{f,i}$ | Road distance between facility $f$ and sequestration site $i$ |
| $\text{rs\_time}_{f,i}$ | Travel duration between facility $f$ and sequestration site $i$ |

Scalars are as follows:

| | |
|---|---|
| **Cost (in 2019 $)** | |
| ad_fc_int | AD fixed cost intercept |
| ad_fc_slope$_1$ | AD fixed cost slope below threshold |
| ad_fc_slope$_2$ | AD fixed cost slope above threshold |
| ad_vc_int | AD variable cost intercept |
| ad_vc_slope$_1$ | AD variable cost slope below threshold |
| ad_vc_slope$_2$ | AD variable cost slope above threshold |
| up_fc_int | Biogas upgrading fixed cost intercept |
| up_fc_slope$_1$ | Biogas upgrading fixed cost slope below threshold |
| up_fc_slope$_2$ | Biogas upgrading fixed cost slope above threshold |
| up_vc_int | Biogas upgrading variable cost intercept |
| up_vc_slope$_1$ | Biogas upgrading variable cost slope below threshold |
| up_vc_slope$_2$ | Biogas upgrading variable cost slope above threshold |
| inj_fc_int | RNG injection fixed cost intercept |
| inj_fc_slope$_1$ | RNG injection fixed cost slope below threshold |
| inj_fc_slope$_2$ | RNG injection fixed cost slope above threshold |
| inj_vc_int | RNG injection variable cost intercept |
| inj_vc_slope$_1$ | RNG injection variable cost slope below threshold |
| inj_vc_slope$_2$ | RNG injection variable cost slope above threshold |
| comp_fc_int$_a$ | $CO_2$ compression to transporting pressure fixed cost intercept |
| comp_fc_slope$_{a1}$ | $CO_2$ compression to transporting pressure fixed cost slope below threshold |
| comp_fc_slope$_{a2}$ | $CO_2$ compression to transporting pressure fixed cost slope above threshold |
| comp_vc_int$_a$ | $CO_2$ compression to transporting pressure variable cost intercept |
| comp_vc_slope$_{a1}$ | $CO_2$ compression to transporting pressure variable cost slope below threshold |
| comp_vc_slope$_{a2}$ | $CO_2$ compression to transporting pressure variable cost slope above threshold |
| comp_fc_int$_b$ | $CO_2$ compression to sequestration pressure fixed cost intercept |
| comp_fc_slope$_{b1}$ | $CO_2$ compression to sequestration pressure fixed cost slope below threshold |
| comp_fc_slope$_{b2}$ | $CO_2$ compression to sequestration pressure fixed cost slope above threshold |
| comp_vc_int$_b$ | $CO_2$ compression to sequestration pressure variable cost intercept |
| comp_vc_slope$_{b1}$ | $CO_2$ compression to sequestration pressure variable cost slope below threshold |
| comp_vc_slope$_{b2}$ | $CO_2$ compression to sequestration pressure variable cost slope above threshold |
| cap_fc_int | $CO_2$ capture fixed cost intercept |
| cap_fc_slope$_1$ | $CO_2$ capture fixed cost slope below threshold |
| cap_fc_slope$_2$ | $CO_2$ capture fixed cost slope above threshold |
| cap_vc_int | $CO_2$ capture variable cost intercept |
| cap_vc_slope$_1$ | $CO_2$ capture variable cost slope below threshold |
| cap_vc_slope$_2$ | $CO_2$ capture variable cost slope above threshold |
| monitoring | $CO_2$ storage monitoring cost |
| fs_mi | Feedstock transport cost per mile |
| fs_hr | Feedstock transport cost per hour |
| rs_mi | $CO_2$ transport cost per mile |
| rs_hr | $CO_2$ transport cost per hour |
| | |
| **Revenues ($/mmbtu)** | |
| lcfs | LCFS credit price |
| d5 | RIN D5 credit price |
| cellulosic_waiver | Cellulosic waiver price |
| 45q | 45Q tax credit |
| rng | RNG price |
| | |
| **Other assumptions** | |
| ch4_yield | $CH_4$ volume percentage in biogas |
| baseline_ci | Baseline carbon intensity of RNG |
| irr | Internal rate of return |
| life | Project lifetime (years) |
| crf | Capital Recovery Factor = $\frac{\mathrm{irr}\times(1+\mathrm{irr})^{\mathrm{life}}}{(1+\mathrm{irr})^{\mathrm{life}}-1}$ |
| electricity | Grid electricity carbon intensity |
| transport | Transport emissions |
| compression$_a$ | $CO_2$ compression work to transporting pressure |
| compression$_b$ | $CO_2$ compression work to sequestration pressure |
| co2_truckload | $CO_2$ transport truck capacity |
| fs_truckload | Feedstock transport truck capacity |

Decision variables are as follows:

| | |
|---|---|
| $\text{ad}_f$ | Binary if facility $f$ is active |
| $\text{seq}_i$ | Binary if sequestration site $i$ is active |
| $\text{q\_feed}_{s,f,t}$ | Quantity of feedstock from source $s$ of type $t$ delivered to facility $f$ |
| $\text{q\_feedf}_f$ | Total quantity of feedstock used at facility $f$ <br> $= \sum_{s,t} \text{q\_feed}_{s,f,t}$ |
| $\text{q\_feedf\_nowwtp}_f$ | Total quantity of feedstock used at facility $f$, excluding wastewater <br> $= \sum_{s,t} \text{q\_feed}_{s,f,t} - \text{q\_feed}_{s,f,t=\text{wastewater}} \times \text{ton}_{t=\text{wastewater}}$ |
| $\text{q\_ch4}_{t,f}$ | Quantity of $CH_4$ from feedstock type $t$ at facility $f$ <br> $= \sum_{s} \text{q\_feed}_{s,f,t} \times \text{ts}_t \times \text{vs}_t \times \text{biogas\_yield}_t \times \text{ch4\_yield}$ |
| $\text{q\_ch4f}_f$ | Quantity of $CH_4$ produced at facility $f$ <br> $\sum_t \text{q\_ch4}_{t,f}$ |
| $\text{q\_captf}_f$ | Quantity of $CO_2$ captured at facility $f$ <br> $= \sum_{s,t} \text{q\_feed}_{s,f,t} \times \text{ts}_t \times \text{vs}_t \times \text{biogas\_yield}_t \times (1 - \text{ch4\_yield})$ |
| $\text{q\_co2seq}_i$ | Quantity of $CO_2$ sequestered at sequestration site $i$ |
| $\text{q\_co2trans}_{f,i}$ | Quantity of $CO_2$ transported from facility $f$ to sequestration site $i$ |

## Model

**Objective Function.** We aim to minimize net cost over the project lifetime:

$$\min \text{net cost} = \text{life} \times (\text{total cost} - \text{total revenue}) \tag{3}$$

where total cost is defined as:

$$\begin{aligned}
\text{total cost} = &\sum_c \Big\{ (\text{ad}_c \times (\sum_{i=1}^{n} \vec{\textbf{Intc}}_i) + \\
&\vec{\textbf{ad_fc}} \times \text{q_feedf_nowwtp}_c + \vec{\textbf{ad_vc}} \times \text{q_feedf}_c + \\
&\vec{\textbf{up_inj}} \times \text{q_ch4f}_c + \vec{\textbf{comp_capt}} \times \text{q_captf}_c + \\
&\text{lcfs} \times \text{compression}_a \times \text{electricity} \times \text{q_captf}_c \Big\} + \\
&\sum_l \Big\{ (\text{ad}_l \times (\sum_{i=1}^{n} \vec{\textbf{Intl}}_i)) + \\
&\vec{\textbf{up_inj}} \times \text{q_ch4f}_l + \vec{\textbf{comp_capt}} \times \text{q_captf}_l + \\
&\text{lcfs} \times \text{compression}_a \times \text{electricity} \times \text{q_captf}_l \Big\} + \\
&\sum_{s,f,t} \Big\{ (\text{fs_dist}_{s,f} \times \text{fs_mi} + \text{fs_time}_{s,f} * \text{fs_hr}) \times \frac{\text{q_feed}_{s,f,t}}{\text{fs_truckload}} + \\
&\text{per_ton}_{s,f} \times \text{q_feed}_{s,f,t} \Big\} + \\
&\sum_{f,i} \Big\{ (\text{rs_time}_{f,i} \times \text{rs_hr} + \text{rs_dist}_{f,i} \times \text{rs_mi}) \times \frac{\text{q_co2trans}_{f,i}}{\text{co2_truckload}} + \\
&\text{lcfs} \times \text{transport} \times \text{q_co2trans}_{f,i} \times \text{rs_dist}_{f,i} \Big\} + \\
&\sum_i \Big\{ (\text{seq}_i \times ((\text{injection_fc}_i + \text{seismic}_i) \times \text{crf} + \text{injection_vc}_i)) + \\
&\vec{\textbf{comp_mon}} \times \text{q_co2seq}_i + \text{lcfs} \times \text{compression}_b \times \text{electricity} \times \text{q_co2seq}_i \Big\}
\end{aligned} \tag{4}$$

and total revenue is defined as:

$$\begin{aligned}
\text{total revenue} = &\sum_{c}\Big\{\text{q_ch4f}_c \times (\text{rng} + \text{d5})\Big\} + \sum_{l}\Big\{\text{q_ch4f}_l \times (\text{rng} + \text{d5} + \text{cellulosic})\Big\} + \\
&\sum_{t,f}\Big\{\text{q_ch4}_{t,f} \times [\text{lcfs} \times (\text{baseline_ci} - \text{c_intensity}_t)]\Big\} + \\
&\sum_{f}\Big\{\text{q_captf}_f \times \vec{\mathbf{45q}}\Big\} + \\
&\sum_{i}\Big\{\text{q_co2seq}_i \times (\text{lcfs})\Big\}
\end{aligned} \tag{5}$$

We denote $\vec{\mathbf{Intc}}$ to be a vector of all piecewise intercepts relevant to the total costs for codigesting facilities and $\vec{\mathbf{Intl}}_l$ to be a vector of all piecewise intercepts relevant to the total costs for landfills:

$$\vec{\mathbf{Intc}} = \begin{bmatrix} \text{ad\_fc\_int} \times \text{crf} \\ \text{ad\_vc\_int} \\ \text{up\_fc\_int} \times \text{crf} \\ \text{up\_vc\_int} \\ \text{inj\_fc\_int} \times \text{crf} \\ \text{inj\_vc\_int} \\ \text{comp\_fc\_int}_a \times \text{crf} \\ \text{comp\_vc\_int}_a \\ \text{cap\_fc\_int} \times \text{crf} \\ \text{cap\_vc\_int} \\ \text{pipe\_fc}_c \times \text{crf} \\ \text{pipe\_vc}_c \end{bmatrix} \qquad \vec{\mathbf{Intl}} = \begin{bmatrix} \text{lmop}_l \\ \text{up\_fc\_int} \times \text{crf} \\ \text{up\_vc\_int} \\ \text{inj\_fc\_int} \times \text{crf} \\ \text{inj\_vc\_int} \\ \text{comp\_fc\_int}_a \times \text{crf} \\ \text{comp\_vc\_int}_a \\ \text{cap\_fc\_int} \times \text{crf} \\ \text{cap\_vc\_int} \\ \text{pipe\_fc}_l \times \text{crf} \\ \text{pipe\_vc}_l \end{bmatrix}$$

We denote $\vec{\mathbf{ad\_fc}}$ and $\vec{\mathbf{ad\_vc}}$ to be vectors of the piecewise slopes for fixed and variable costs for anaerobic digesters, taking on different values depending on the value of $\text{q\_feed}_{s,f,t}$.

$$\vec{\mathbf{ad\_fc}} = \begin{bmatrix} \text{ad\_fc\_slope}_1 \\ \text{ad\_fc\_slope}_2 \end{bmatrix} \times \text{crf} \qquad \vec{\mathbf{ad\_vc}} = \begin{bmatrix} \text{ad\_vc\_slope}_1 \\ \text{ad\_vc\_slope}_2 \end{bmatrix}$$

We denote $\vec{\mathbf{up\_inj}}$ and $\vec{\mathbf{comp\_capt}}$ to be vectors of the piecewise slopes for fixed and variable costs for upgrading and injection, and compression and $CO_2$ capture, respectively. Facilities take on different values within these vectors depending on the values of $\text{q\_captf}_f$ and $\text{q\_ch4f}_f$.

$$\vec{\mathbf{up\_inj}} = \begin{bmatrix} (\text{up\_fc\_slope}_1 + \text{inj\_fc\_slope}_1) \times \text{crf} + \text{up\_vc\_slope}_1 + \text{inj\_vc\_slope}_1 \\ (\text{up\_fc\_slope}_2 + \text{inj\_fc\_slope}_2) \times \text{crf} + \text{up\_vc\_slope}_2 + \text{inj\_vc\_slope}_2 \end{bmatrix}$$

$$\vec{\mathbf{comp\_capt}} = \begin{bmatrix} (\text{comp\_fc\_slope}_{a1} + \text{capt\_fc\_slope}_1) \times \text{crf} + \text{comp\_vc\_slope}_{a1} + \text{capt\_vc\_slope}_1 \\ (\text{comp\_fc\_slope}_{a2} + \text{capt\_fc\_slope}_2) \times \text{crf} + \text{comp\_vc\_slope}_{a2} + \text{capt\_vc\_slope}_2 \end{bmatrix}$$

We denote $\vec{\mathbf{comp\_mon}}$ to be vectors of the piecewise slopes for fixed and variable costs of monitoring and compression cost at sequestration sites. Sequestration sites take on values within these vectors depending on the value of $\text{q\_co2seq}_i$.

$$\vec{\mathbf{comp\_mon}} = \begin{bmatrix} \text{comp\_fc\_slope}_{b1} \times \text{crf} + \text{comp\_vc\_slope}_{b1} + \text{monitoring} \\ \text{comp\_fc\_slope}_{b2} \times \text{crf} + \text{comp\_vc\_slope}_{b2} + \text{monitoring} \end{bmatrix}$$

We denote $\vec{\mathbf{45q}}$ to be a vector of the piecewise values for the 45Q tax credits around the threshold of 100,000 $tCO_2$/year.

$$\vec{\mathbf{45q}} = \begin{bmatrix} 0 \\ 50 \end{bmatrix}$$

**Constraints**. The objective function is subject to:

Feedstock used is zero if the facility is not activated

$$\text{q\_feed}_{s,f,t} \leq \text{supply}_{s,t} \times \text{ad}_f \tag{6}$$

Feedstock used cannot exceed available supply

$$\sum_f \text{q\_feed}_{s,f,t} = \text{supply}_{s,t} \tag{7}$$

$CO_2$ transported is equal to $CO_2$ captured

$$\sum_i \text{q\_co2trans}_{f,i} = \text{q\_captf}_f \tag{8}$$

$CO_2$ sequestered is equal to $CO_2$ transported

$$\sum_f \text{q\_co2trans}_{f,i} = \text{q\_co2seq}_i \tag{9}$$

$CO_2$ sequestered cannot be more than available capacity

$$\text{q\_co2seq}_i \leq \text{capacity}_i \times \text{seq}_i \tag{10}$$

Minimum sequestration volume

$$\text{q\_co2seq}_i \geq 25000 \times \text{seq}_i \tag{11}$$

## References


[1] CalFire. Incorporated cities. URL https://frap.fire.ca.gov/mapping/gis-data/.

[2] Caltrans. City boundaries. URL https://gisdata-caltrans.opendata.arcgis.com/search?tags=Boundaries. Library Catalog: gisdata-caltrans.opendata.arcgis.com.

[3] California geological survey, . URL https://www.conservation.ca.gov/cgs.

[4] Hanna Marie Breunig, Tyler Huntington, Ling Jin, Alastair Robinson, and Corinne Donahue Scown. Temporal and geographic drivers of biomass residues in california. 139:287–297. ISSN 0921-3449. doi: 10.1016/j.resconrec.2018.08.022. URL http://www.sciencedirect.com/science/article/pii/S0921344918303148.

[5] Filomena Ardolino and Umberto Arena. Biowaste-to-biomethane: An LCA study on biogas and syngas roads. 87:441–453. ISSN 0956-053X. doi: 10.1016/j.wasman.2019.02.030. URL http://www.sciencedirect.com/science/article/pii/S0956053X19301011.

[6] Overview | places API, . URL https://developers.google.com/places/web-service/overview. Library Catalog: developers.google.com.

[7] Nathan Parker, Robert Williams, Rosa Dominguez-Faus, and Daniel Scheitrum. Renewable natural gas in california: An assessment of the technical and economic potential. 111:235–245. ISSN 0301-4215. doi: 10.1016/j.enpol.2017.09.034. URL http://www.sciencedirect.com/science/article/pii/S0301421517305955.

[8] David L. McCollum and Joan M. Ogden. Techno-economic models for carbon dioxide compression, transport, and storage & correlations for estimating carbon dioxide density and viscosity. URL https://escholarship.org/uc/item/1zg00532.

[9] Peter C. Psarras, Stephen Comello, Praveen Bains, Panunya Charoensawadpong, Stefan Reichelstein, and Jennifer Wilcox. Carbon capture and utilization in the industrial sector. 51(19):11440–11449. ISSN 1520-5851. doi: 10.1021/acs.est.7b01723.

[10] Yeqing Li, Ruihong Zhang, Guangqing Liu, Chang Chen, Yanfeng He, and Xiaoying Liu. Comparison of methane production potential, biodegradability, and kinetics of different organic substrates. 149:565–569. ISSN 0960-8524. doi: 10.1016/j.biortech.2013.09.063. URL http://www.sciencedirect.com/science/article/pii/S0960852413014958.

[11] Humberto Escalante, Liliana Castro, Paola Gauthier-Maradei, and Reynel Rodríguez De La Vega. Spatial decision support system to evaluate crop residue energy potential by anaerobic digestion. 219:80–90. ISSN 0960-8524. doi: 10.1016/j.biortech.2016.06.136. URL http://www.sciencedirect.com/science/article/pii/S0960852416309609.

[12] California Department of Food {and} Agriculture. Agricultural overview. URL http://www.cdfa.ca.gov/Statistics/PDFs/AgResourceDirectory2008/1_2008_OverviewSection.pdf.

[13] Qie Sun, Hailong Li, Jinying Yan, Longcheng Liu, Zhixin Yu, and Xinhai Yu. Selection of appropriate biogas upgrading technology-a review of biogas cleaning, upgrading and utilisation. 51:521–532. ISSN 1364-0321. doi: 10.1016/j.rser.2015.06.029. URL http://www.sciencedirect.com/science/article/pii/S1364032115006012.

[14] Matthew D Ong, Robert B Williams, and Stephen R Kaffka. Comparative assessment of technology options for biogas clean-up. page 161.

[15] Daniel L. Sanchez, Nils Johnson, Sean T. McCoy, Peter A. Turner, and Katharine J. Mach. Near-term deployment of carbon capture and sequestration from biorefineries in the united states. 115(19):4875–4880. ISSN 0027-8424, 1091-6490. doi: 10.1073/pnas.1719695115. URL https://www.pnas.org/content/115/19/4875. Publisher: National Academy of Sciences Section: Physical Sciences.

[16] NATCARB/ATLAS, . URL https://www.netl.doe.gov/coal/carbon-storage/strategic-program-support/natcarb-atlas. Library Catalog: www.netl.doe.gov.

[17] J. Ogden and N. Johnson. Techno-economic analysis and modeling of carbon dioxide (CO2) capture and storage (CCS) technologies. In M. Mercedes Maroto-Valer, editor, *Developments and Innovation in Carbon Dioxide (CO2) Capture and Storage Technology*, volume 1 of *Woodhead Publishing Series in Energy*, pages 27–63. Woodhead Publishing. ISBN 978-1-84569-533-0. doi: 10.1533/9781845699574.1.27. URL http://www.sciencedirect.com/science/article/pii/B9781845695330500023.

[18] Sean T. McCoy. The economics of CO2 transport by pipeline and storage in saline aquifers and oil reservoirs. doi: 10.1184/R1/6073547.v1. URL https://kilthub.cmu.edu/articles/journal_contribution/The_Economics_of_CO_sub_2_sub_Transport_by_Pipeline_and_Storage_in_Saline_Aquifers_and_Oil_Reservoirs/6073547. Publisher: Carnegie Mellon University.

[19] Jan Martin Nordbotten, Michael A. Celia, and Stefan Bachu. Injection and storage of CO2 in deep saline aquifers: Analytical solution for CO2 plume evolution during injection. 58(3): 339–360. ISSN 1573-1634. doi: 10.1007/s11242-004-0670-9. URL https://doi.org/10.1007/s11242-004-0670-9.

[20] Ting Horng Chung, Mohammad Ajlan, Lloyd L. Lee, and Kenneth E. Starling. Generalized multiparameter correlation for nonpolar and polar fluid transport properties. URL https://pubs.acs.org/doi/10.1021/ie00076a024.

[21] Michael Batzle and Zhijing Wang. Seismic properties of pore fluids. 57(11):1396–1408. ISSN 0016-8033, 1942-2156. doi: 10.1190/1.1443207. URL http://library.seg.org/doi/10.1190/1.1443207.
